# Supplementary material for: Discrete tensor product BGG sequences: splines and finite elements
Source: arXiv:2302.02434 source file (2023-12-30)
Supplement: Supplementary file 1 [file old_proof_appendix.tex]

We prove the result by induction on $m$. 
First, we verify the identity for $m=1$. In fact, let $\{e_{l}\}_{l=1}^{n}$ be the dual basis to $\{dx^{k}\}_{k=1}^{n}$, i.e., $dx^{k}(e_{l})=\delta_{kl}$. Let $\rho$ be any vector of $k+1$ indices in $\{1,\dots,n\}$. Once we have shown that the identity holds if applied to $(e_{\rho_1},\dots,e_{\rho_{k+1}})$, it holds by linearity. Let $\sigma\in\Sigma(k,n)$ and $\tau\in\{1,\dots,n\}$. First, we use the definition of $s^{k,m}$ in equation~\eqref{def:s}.
\remove{\begin{align*}
&s^{k, 1}(dx^{1}\wedge\cdots \wedge dx^{k}\otimes dx^{k+1})(e_{\sigma_1}, \cdots, e_{\sigma_{k+1}})(\cdot)\\
&=\sum_{l=1}^{k+1}(-1)^{l+1}dx^{1}\wedge \cdots \wedge dx^{k}\otimes dx^{k+1}(e_{\sigma_{1}}, \cdots, \widehat{e_{\sigma_{l}}}, \cdots, e_{\sigma_{k+1}})(e_{{\sigma_{l}}})\\
&=\sum_{l=1}^{k+1}(-1)^{l+1} dx^{k+1}(e_{\sigma_l})dx^{1}\wedge \cdots \wedge dx^{k}(e_{\sigma_{1}}, \cdots, \widehat{e_{\sigma_{l}}}, \cdots, e_{\sigma_{k+1}})\\
&= dx^{k+1}\wedge dx^{1}\wedge\cdots \wedge dx^{k}\otimes 1(e_{{\sigma_{1}}}, \cdots, e_{\sigma_{k+1}})(\cdot),
\end{align*}}

\begin{align*}
s^{k, 1}(dx^{\sigma}\otimes dx^{\tau})(e_{\rho_1}, \cdots, e_{\rho_{k+1}})()
&=\sum_{l=1}^{k+1}(-1)^{l+1}dx^{\sigma}\otimes dx^{\tau}(e_{\rho_{1}}, \cdots, \widehat{e_{\rho_{l}}}, \cdots, e_{\rho_{k+1}})(e_{{\rho_{l}}})\\
&= \sum_{l=1}^{k+1}(-1)^{l+1}
dx^\sigma(e_{\rho_{1}}, \cdots, \widehat{e_{\rho_{l}}}, \cdots, e_{\rho_{k+1}}) \,dx^\tau(e_{{\rho_{l}}}),
\end{align*}
where the second equality is by the definition of the tensor product.
Clearly, the term under the sum can only be nonzero, if the indices in the argument to $dx^\sigma$ are a permutation of $\sigma$ and if $\rho_l = \tau$. Define $\tilde\rho = (\tau,\sigma_1,\dots,\sigma_k)$, then there holds
\begin{gather*}
    s^{k, 1}(dx^{\sigma}\otimes dx^{\tau})(e_{\rho_1}, \cdots, e_{\rho_{k+1}})()
    = \begin{cases}
    \sign \pi & \text{if } \rho = \pi\tilde \rho,\\
    0&\text{else},
    \end{cases}
\end{gather*}
where $\pi$ is any permutation of the entries of $\tilde\rho$. On the other hand, by direct computation,
\begin{gather*}
 [dx^{\tau}\wedge dx^{\sigma}]\otimes 1(e_{{\rho_{1}}}, \cdots, e_{\rho_{k+1}})()
     = \begin{cases}
    \sign \pi & \text{if } \rho = \pi\tilde \rho,\\
    0&\text{else}.
    \end{cases}
\end{gather*}
This implies that 
$$
s^{k, 1}(dx^{\sigma}\otimes dx^{\tau})
=[dx^\tau\wedge dx^\sigma]\otimes 1,
$$
and thus our assumption for $m=1$.

The next step is to assume that the conclusion holds for $m$, and verify the results for $m+1$. In this case, we have $s^{k, m+1}: \alt^{k, m+1}\to \alt^{k+1, m}$. Let $\sigma\in\Sigma(k,n)$, $\tau\in\Sigma(m,n)$ and $\theta\in\{1,\dots,n\}$. Then,
\gkfatal{Only until purple text is finished}
\begin{align*}
&\quad s^{k,m+1}(dx^\sigma\otimes dx^\theta\wedge dx^\tau) (e_{\rho_1}\cdots, e_{\rho_{k+1}})(e_{\rho_{k+2}}, \cdots, e_{\rho_{k+m+1}})\\
&=\sum_{l=1}^{k+1}(-1)^{l+1}(dx^\sigma\otimes dx^\theta\wedge dx^{\tau})
%\\&\quad\quad \quad\quad\quad\quad\quad\quad
(e_{\rho_{1}}, \cdots,  \widehat{e_{\rho_{l}}}, \cdots, e_{\rho_{k+1}})(e_{\rho_{l}}, e_{\rho_{k+2}}, \cdots, e_{\rho_{k+m+1}})\\
&\color{purple}=\sum_{l=1}^{k+1}(-1)^{l+1}dx^{\theta}(e_{\rho_{l}})(dx^\sigma\otimes dx^\tau)
%\\&\quad \quad\quad \quad\quad\quad\quad\quad\quad
(e_{\rho_{1}}, \cdots,  \widehat{e_{\rho_{l}}}, \cdots, e_{\rho_{k+1}})( e_{\rho_{k+2}}, \cdots, e_{\rho_{k+m+1}})
\\& \quad +\remove{\frac{1}{m+1}}\sum_{l=1}^{k+1}(-1)^{l+1}\sum_{t=2}^{m+1}(-1)^{t+1}dx^{k+1}(e_{\rho_{k+t}})(dx^{1}\wedge\cdots \wedge dx^{k}\otimes dx^{k+2} \wedge \cdots\wedge dx^{k+m+1})\\& \quad \quad\quad \quad\quad\quad\quad\quad\quad(e_{\rho_{1}}, \cdots,  \widehat{e_{\rho_{l}}}, \cdots, e_{\rho_{k+1}})( e_{\rho_{l}}, e_{\rho_{k+2}}, \cdots, \widehat{e_{\rho_{k+t}}},\cdots, e_{\rho_{k+m+1}})\\
&=:I_{1}+I_{2}.
\end{align*}
\remove{\begin{align*}
&\quad s(dx^{1}\wedge\cdots \wedge dx^{k}\otimes dx^{k+1}\wedge \cdots\wedge dx^{k+m+1})(e_{\rho_{1}}, \cdots, e_{\rho_{k+1}})(e_{\rho_{k+2}}, \cdots, e_{\rho_{k+m+1}})\\
&=\sum_{l=1}^{k+1}(-1)^{l+1}(dx^{1}\wedge\cdots \wedge dx^{k}\otimes dx^{k+1}\wedge \cdots\wedge dx^{k+m+1})\\&\quad\quad \quad\quad\quad\quad\quad\quad
(e_{\rho_{1}}, \cdots,  \widehat{e_{\rho_{l}}}, \cdots, e_{\rho_{k+1}})(e_{\rho_{l}}, e_{\rho_{k+2}}, \cdots, e_{\rho_{k+m+1}})\\
&=\remove{\frac{1}{m+1}}\sum_{l=1}^{k+1}(-1)^{l+1}dx^{k+1}(e_{\rho_{l}})(dx^{1}\wedge\cdots \wedge dx^{k}\otimes dx^{k+2} \wedge \cdots\wedge dx^{k+m+1})\\&\quad \quad\quad \quad\quad\quad\quad\quad\quad (e_{\rho_{1}}, \cdots,  \widehat{e_{\rho_{l}}}, \cdots, e_{\rho_{k+1}})( e_{\rho_{k+2}}, \cdots, e_{\rho_{k+m+1}})
\\& \quad +\remove{\frac{1}{m+1}}\sum_{l=1}^{k+1}(-1)^{l+1}\sum_{t=2}^{m+1}(-1)^{t+1}dx^{k+1}(e_{\rho_{k+t}})(dx^{1}\wedge\cdots \wedge dx^{k}\otimes dx^{k+2} \wedge \cdots\wedge dx^{k+m+1})\\& \quad \quad\quad \quad\quad\quad\quad\quad\quad(e_{\rho_{1}}, \cdots,  \widehat{e_{\rho_{l}}}, \cdots, e_{\rho_{k+1}})( e_{\rho_{l}}, e_{\rho_{k+2}}, \cdots, \widehat{e_{\rho_{k+t}}},\cdots, e_{\rho_{k+m+1}})\\
&=:I_{1}+I_{2}.
\end{align*}
}
Now by \eqref{eqn:form},
$$
I_{1}=\remove{\frac{k+1}{m+1}}dx^{k+1}\wedge dx^{1}\wedge\cdots \wedge dx^{k}\otimes dx^{k+2} \wedge \cdots\wedge dx^{k+m+1}(e_{\sigma_{1}}, \cdots, e_{\sigma_{k+1}})( e_{\sigma_{k+2}}, \cdots, e_{\sigma_{k+m+1}}),
$$
and 
\begin{align*}
I_{2}&=\remove{\frac{1}{m+1}}\sum_{t=2}^{m+1}(-1)^{t+1}dx^{k+1}(e_{\sigma_{k+t}})s(dx^{1}\wedge\cdots \wedge dx^{k}\otimes dx^{k+2} \wedge \cdots\wedge dx^{k+m+1})\\&
\quad\quad\quad\quad\quad\quad(e_{\sigma_{1}}, \cdots, e_{\sigma_{k+1}})(e_{\sigma_{k+2}}, \cdots, \widehat{e_{\sigma_{k+t}}},\cdots, e_{\sigma_{k+m+1}})\\&
=\remove{\frac{1}{m+1}}\sum_{t=2}^{m+1}(-1)^{t+1}dx^{k+1}(e_{\sigma_{k+t}})
\\&\quad\quad\quad
\cdot\sum_{l=2}^{m+1}(-1)^{l}\frac{k+1}{m}
dx^{k+l}\wedge dx^{1}\wedge\cdots \wedge dx^{k}\otimes dx^{k+2} \wedge  \cdots\wedge \widehat{dx^{k+l}}\wedge \cdots\wedge dx^{k+m+1})\\&
\quad\quad\quad\quad\quad\quad(e_{\sigma_{1}}, \cdots, e_{\sigma_{k+1}})( e_{\sigma_{k+2}}, \cdots, \widehat{e_{\sigma_{k+t}}},\cdots, e_{\sigma_{k+m+1}})\\
&=\remove{\frac{m}{m+1}\frac{k+1}{m}}\sum_{l=2}^{m+1}(-1)^{l+1}
dx^{k+l}\wedge dx^{1}\wedge\cdots \wedge dx^{k}\otimes dx^{k+1} \wedge  \cdots\wedge \widehat{dx^{k+l}}\wedge \cdots\wedge dx^{k+m+1})\\&\quad\quad\quad\quad\quad\quad(e_{\sigma_{1}}, \cdots, e_{\sigma_{k+1}})( e_{\sigma_{k+2}},\cdots, e_{\sigma_{k+m+1}}).
\end{align*}
Here the first identity is by \eqref{eqn:form}, the second is by the definition of $s$ and the last is by the induction assumption.
This completes the induction.
\color{black}
